# Supplementary material for: Domain Adaptive 3D Pose Augmentation for In-the-wild Human Mesh Recovery
Source: arXiv:2206.10457 source file (2022-09-14)
Supplement: Supplementary file 1 [file supplementary_agora.pdf]

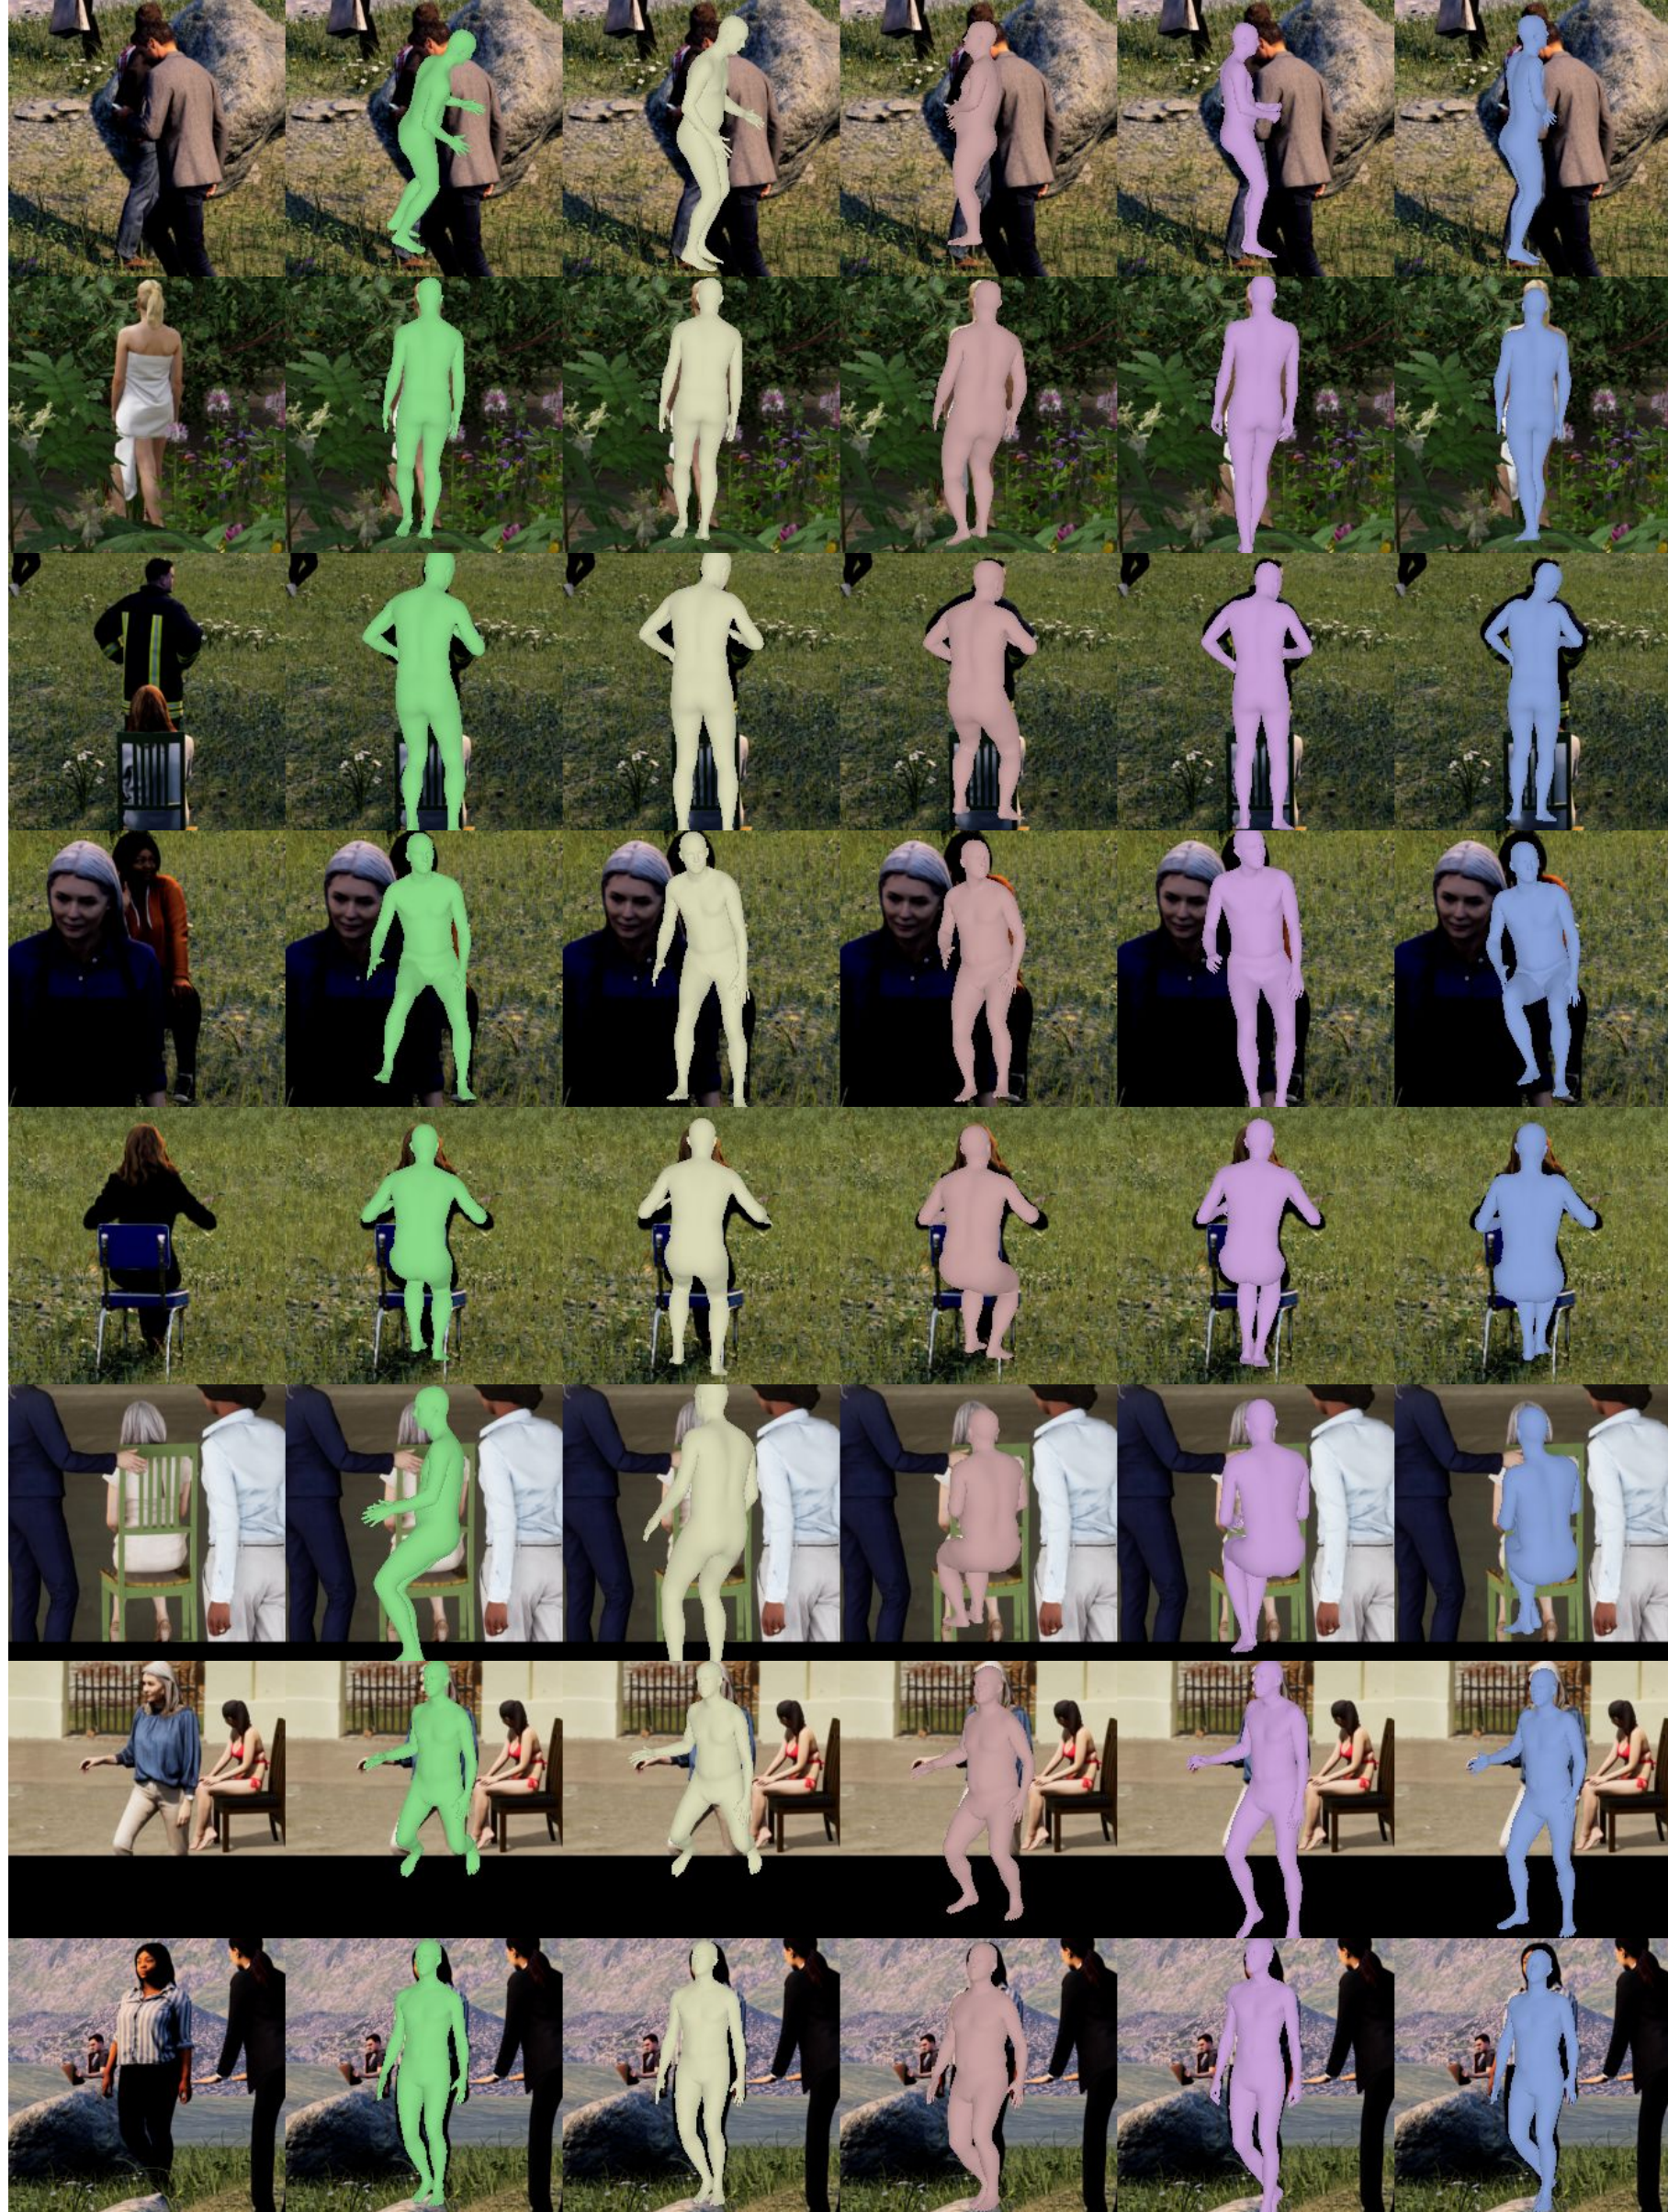

Input

SPIN-pt

SPIN-ft-EFT

SPIN-ft-AGORA-2D

SPIN-ft-AGORA

DAPA (Ours)



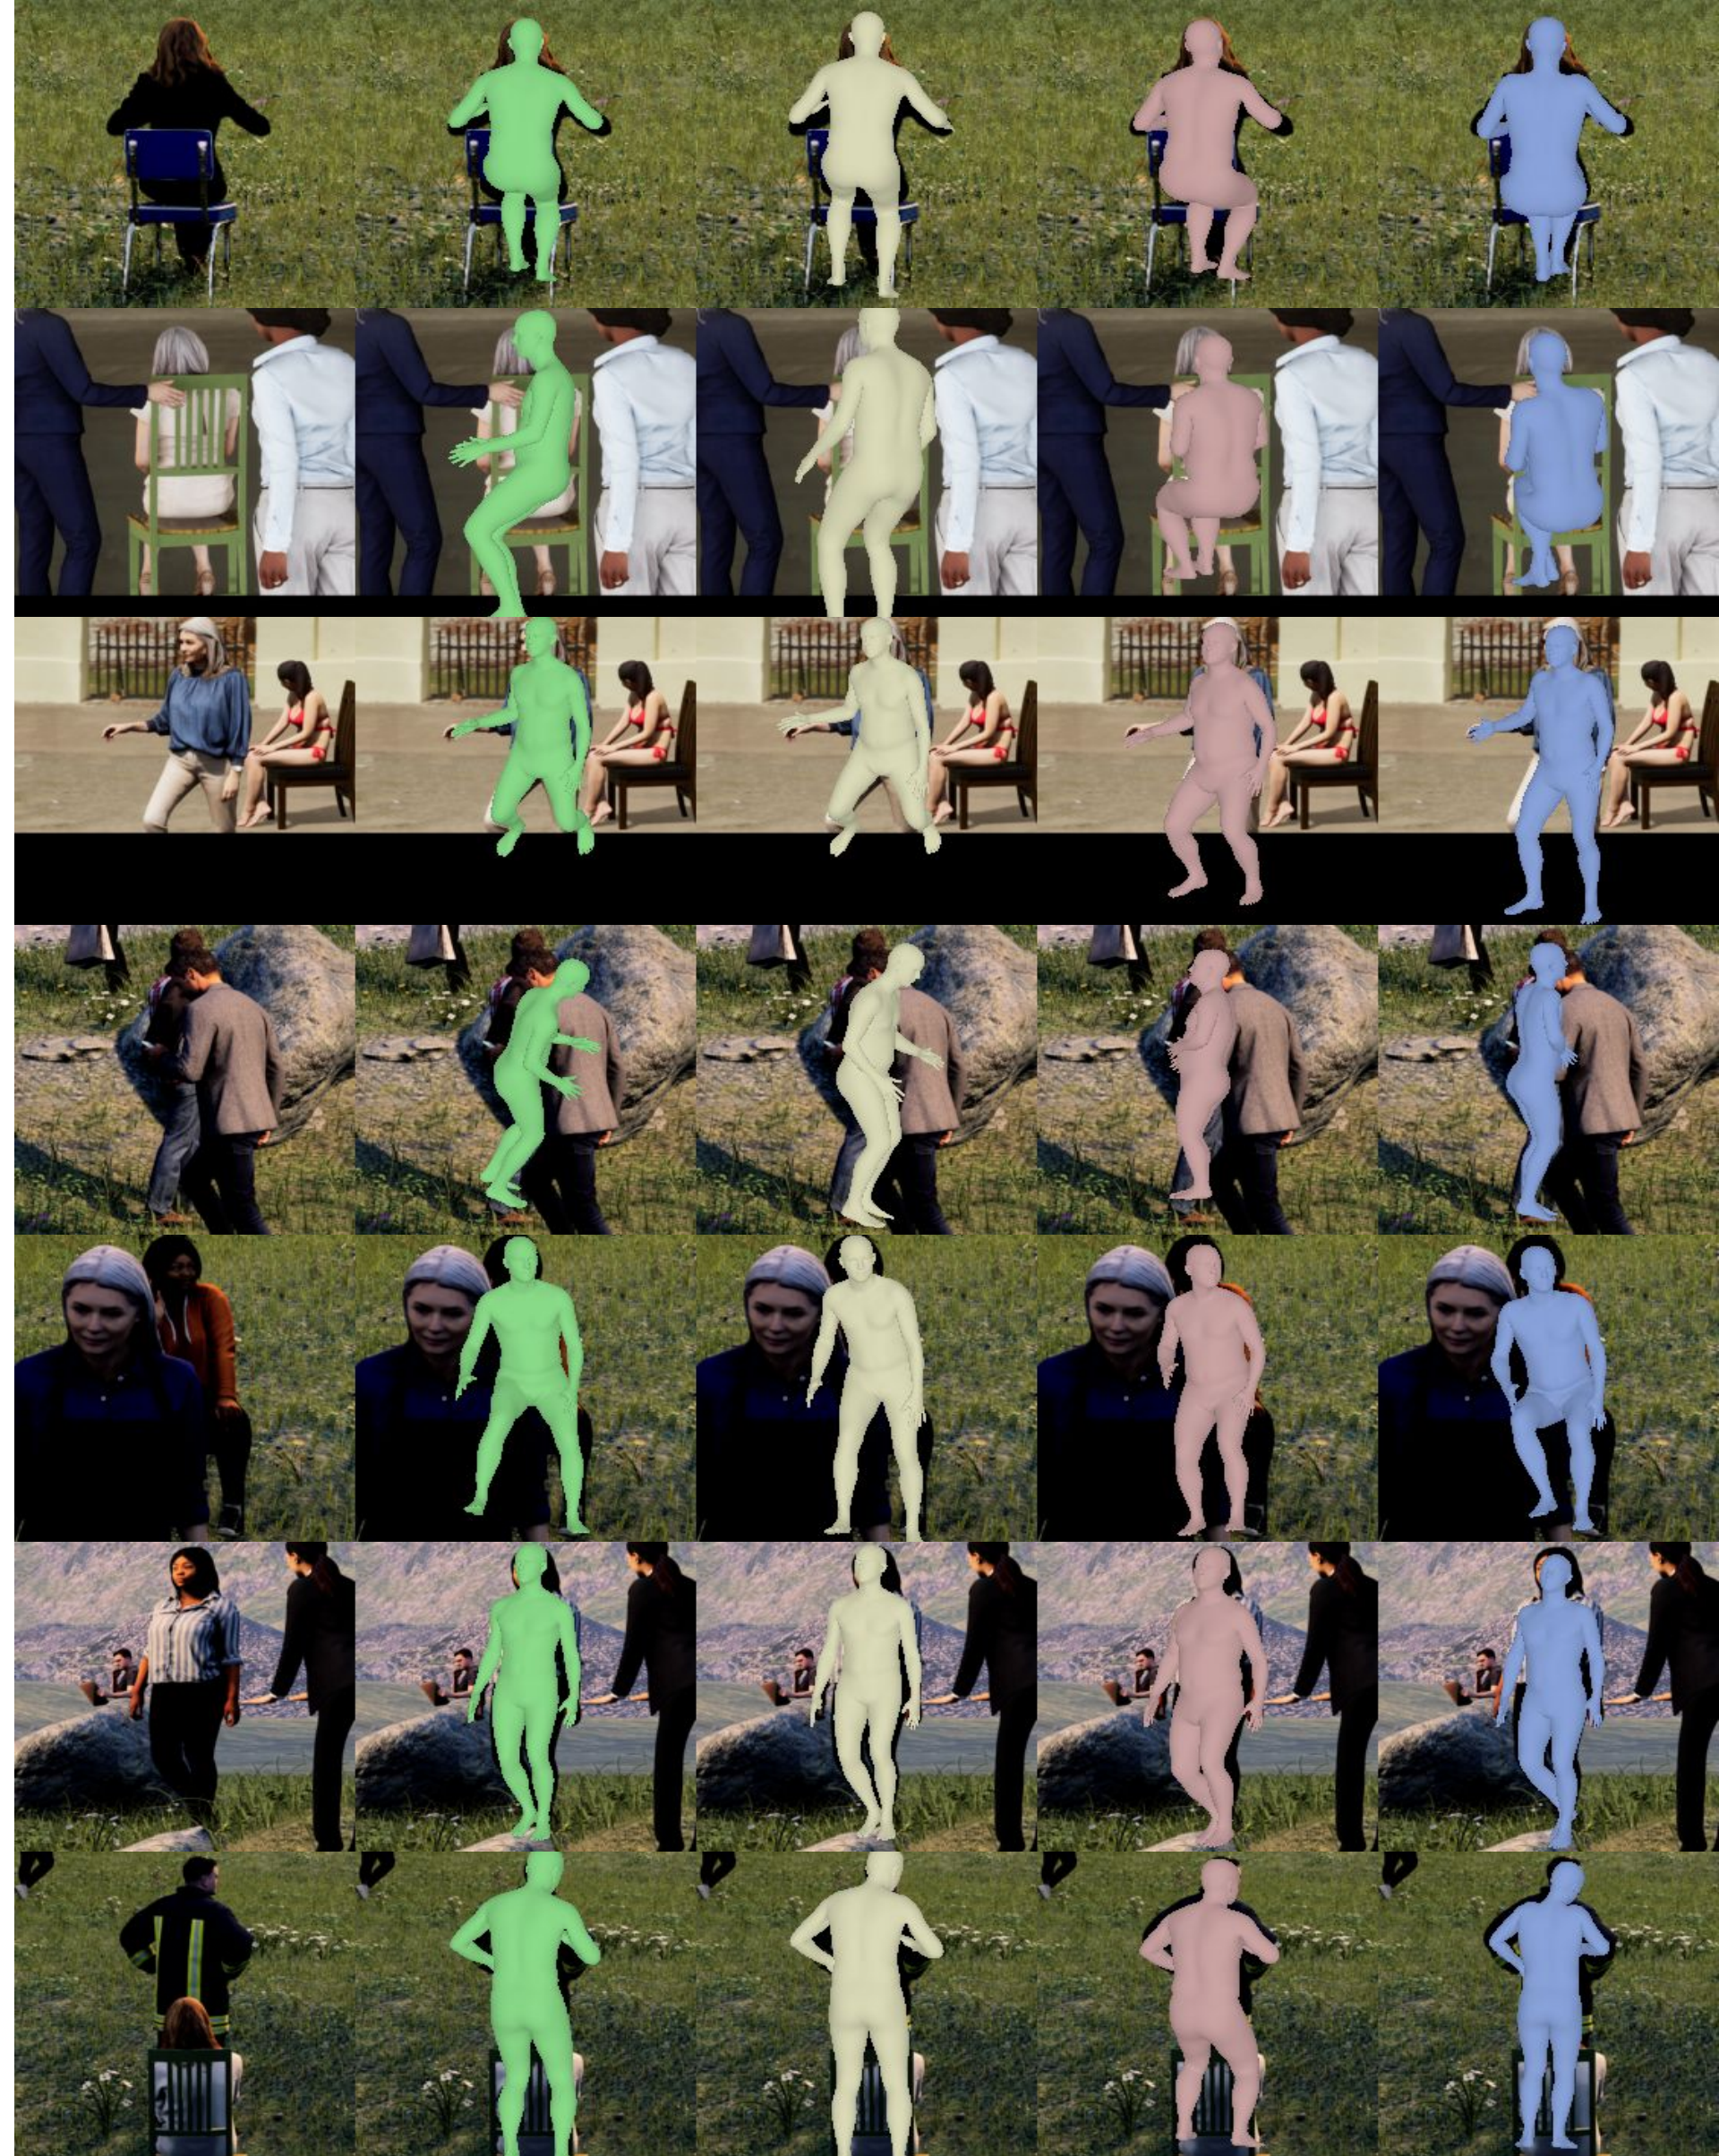

Input

SPIN-pt

SPIN-ft-EFT

SPIN-ft-AGORA-2D

DAPA (Ours)
